# Supplementary material for: Using a Cross-Task Grid of Linear Probes to Interpret CNN Model Predictions On Retinal Images
Source: arXiv:2107.11468 source file (2021-07-23)
Supplement: Supplementary file 1 [file supplement.tex]

%%%%%%%% ICML 2021 EXAMPLE LATEX SUBMISSION FILE %%%%%%%%%%%%%%%%%

\documentclass{article}

% Recommended, but optional, packages for figures and better typesetting:
\usepackage{microtype}
\usepackage{graphicx}
\usepackage{booktabs} % for professional tables
\usepackage[font=small,skip=-2pt]{caption}
%\captionsetup{belowskip=-3pt}

% hyperref makes hyperlinks in the resulting PDF.
% If your build breaks (sometimes temporarily if a hyperlink spans a page)
% please comment out the following usepackage line and replace
% \usepackage{icml2021} with \usepackage[nohyperref]{icml2021} above.
\usepackage{hyperref}

% Attempt to make hyperref and algorithmic work together better:

% Use the following line for the initial blind version submitted for review:
%\usepackage{icml2021}

% If accepted, instead use the following line for the camera-ready submission:
%\usepackage[accepted]{icml2021}

% MINE
\usepackage{subcaption}

% Use the following line for the initial blind version submitted for review:
%\usepackage{icml2021}

% If accepted, instead use the following line for the camera-ready submission:
\usepackage[accepted]{icml2021}

% The \icmltitle you define below is probably too long as a header.
% Therefore, a short form for the running title is supplied here:
%\icmltitlerunning{Using a Cross-Task Grid of Linear Probes to Interpret Retinal Image Predictions}

\begin{document}

\twocolumn[
]

% this must go after the closing bracket ] following \twocolumn[ ...

% This command actually creates the footnote in the first column
% listing the affiliations and the copyright notice.
% The command takes one argument, which is text to display at the start of the footnote.
% The \icmlEqualContribution command is standard text for equal contribution.
% Remove it (just {}) if you do not need this facility.

%\printAffiliationsAndNotice{}  % leave blank if no need to mention equal contribution
% \printAffiliationsAndNotice{}
%\icmlEqualContribution} % otherwise use the standard text.

testing

\end{document}
